# Supplementary material for: TiC-CLIP: Continual Training of CLIP Models
Source: arXiv:2310.16226 source file (2024-03-21)
Supplement: Supplementary file 1 [file barplot_results.tex]

\begin{figure*}[!t]
    \centering
    \begin{subfigure}[b]{\linewidth}
    \includegraphics[width=\linewidth]{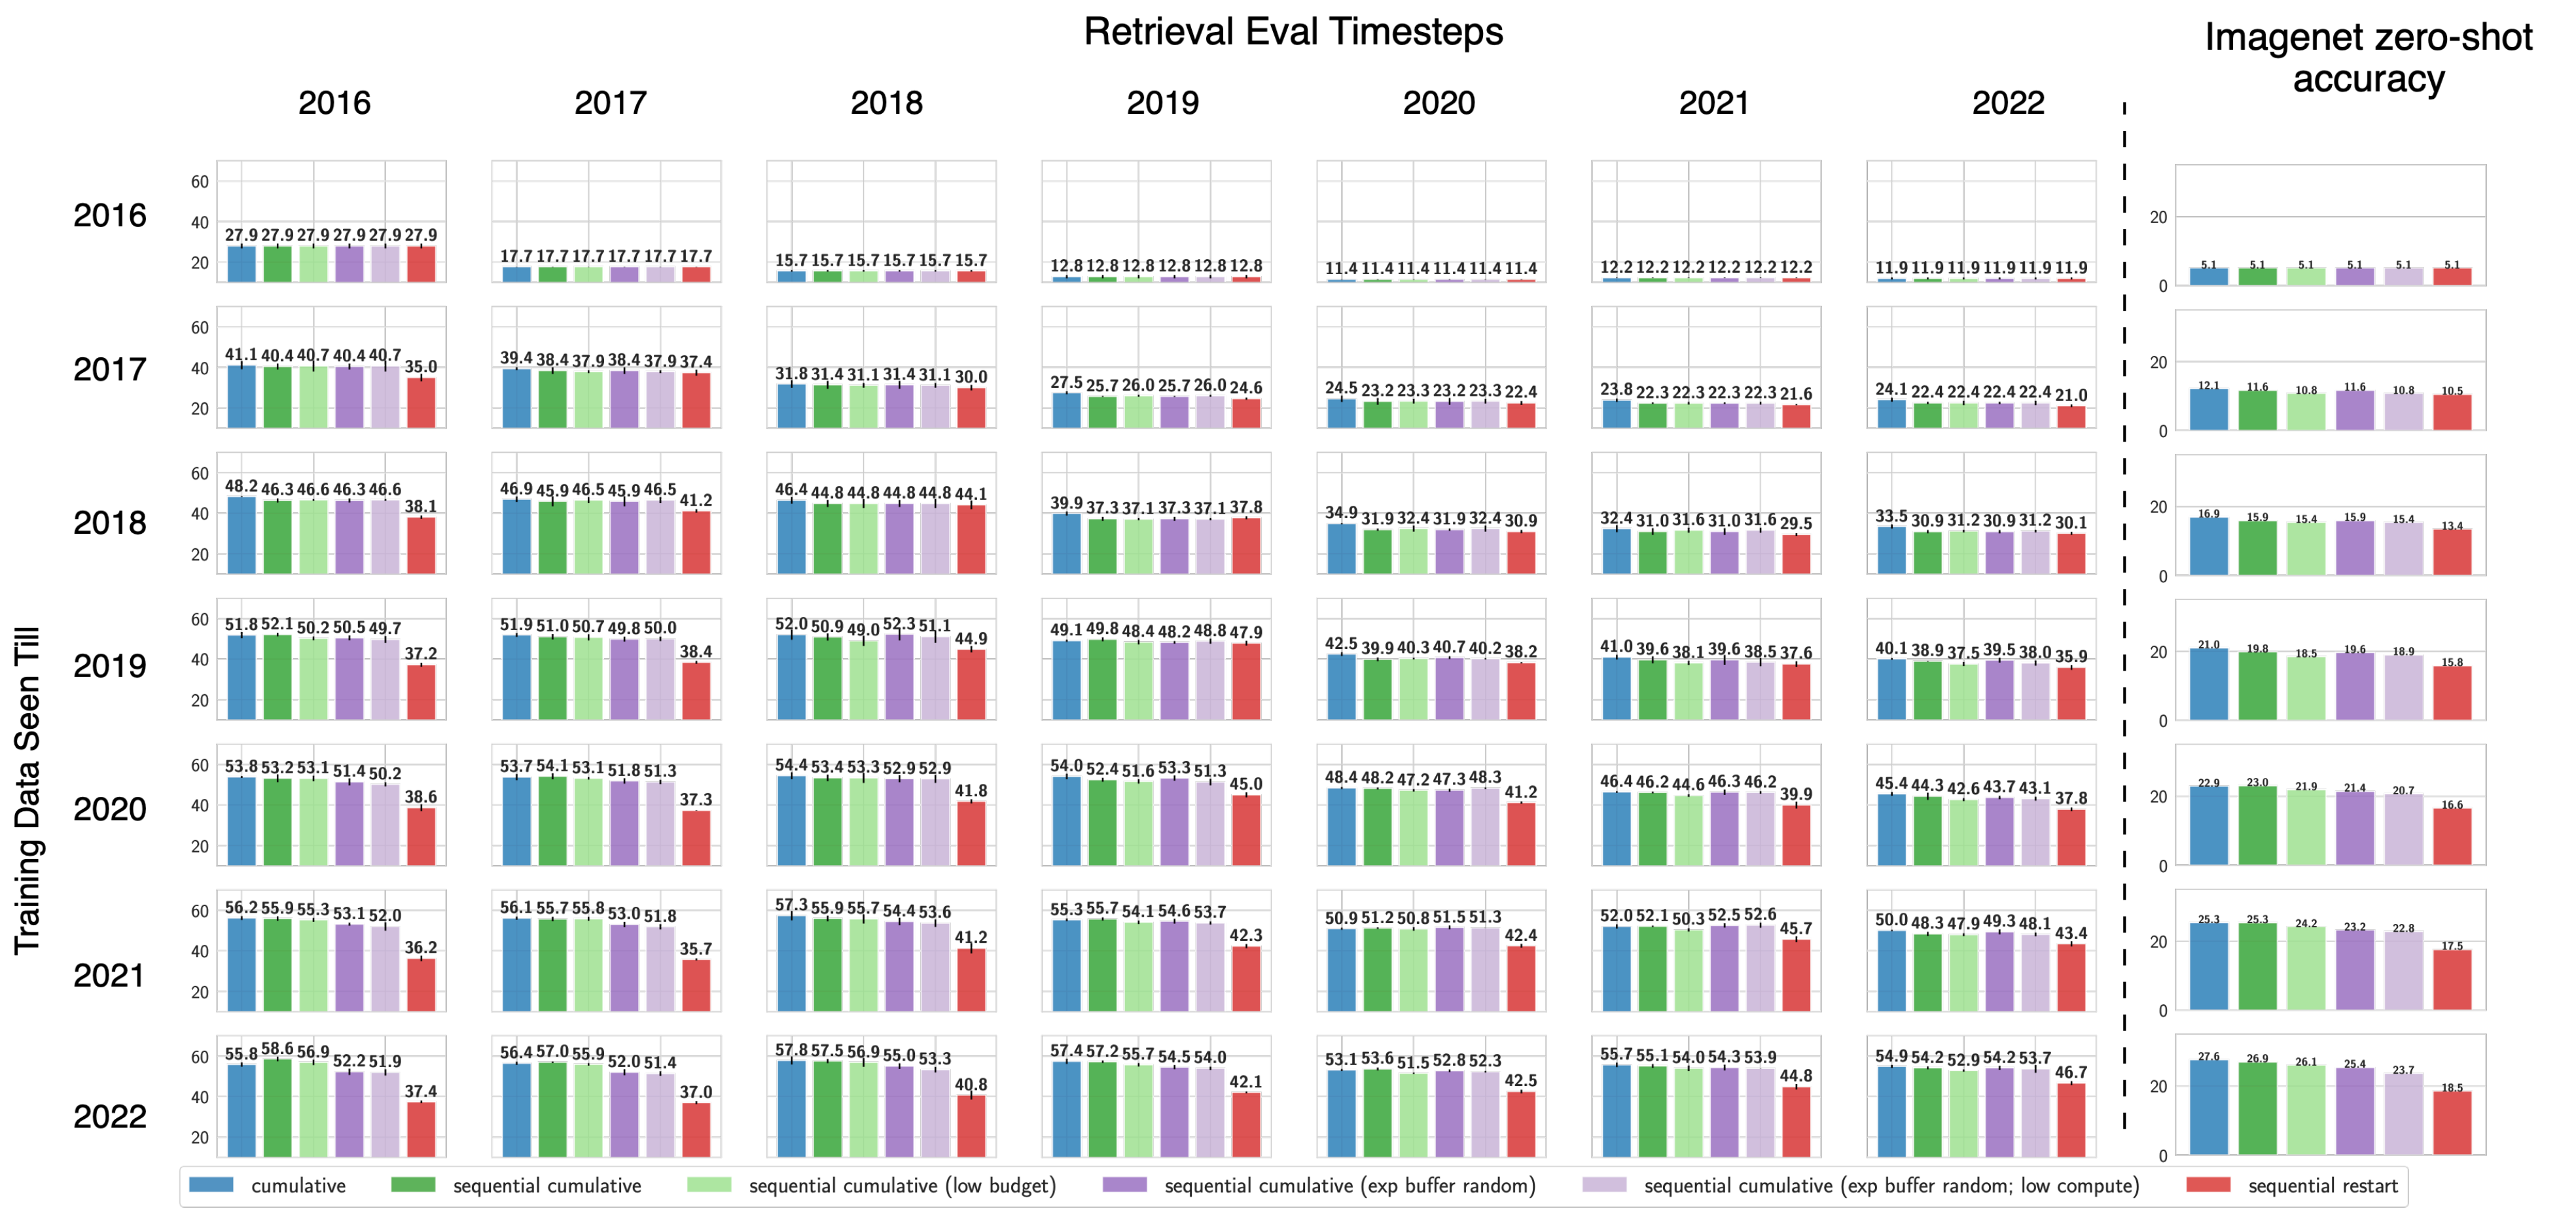} 
     \caption{}   
    \end{subfigure}
    \caption{YFCC 15M results}
    \label{fig:intro-figure}
\end{figure*}

\begin{figure*}[!t]
    \centering
    \begin{subfigure}[b]{\linewidth}
    \includegraphics[width=\linewidth]{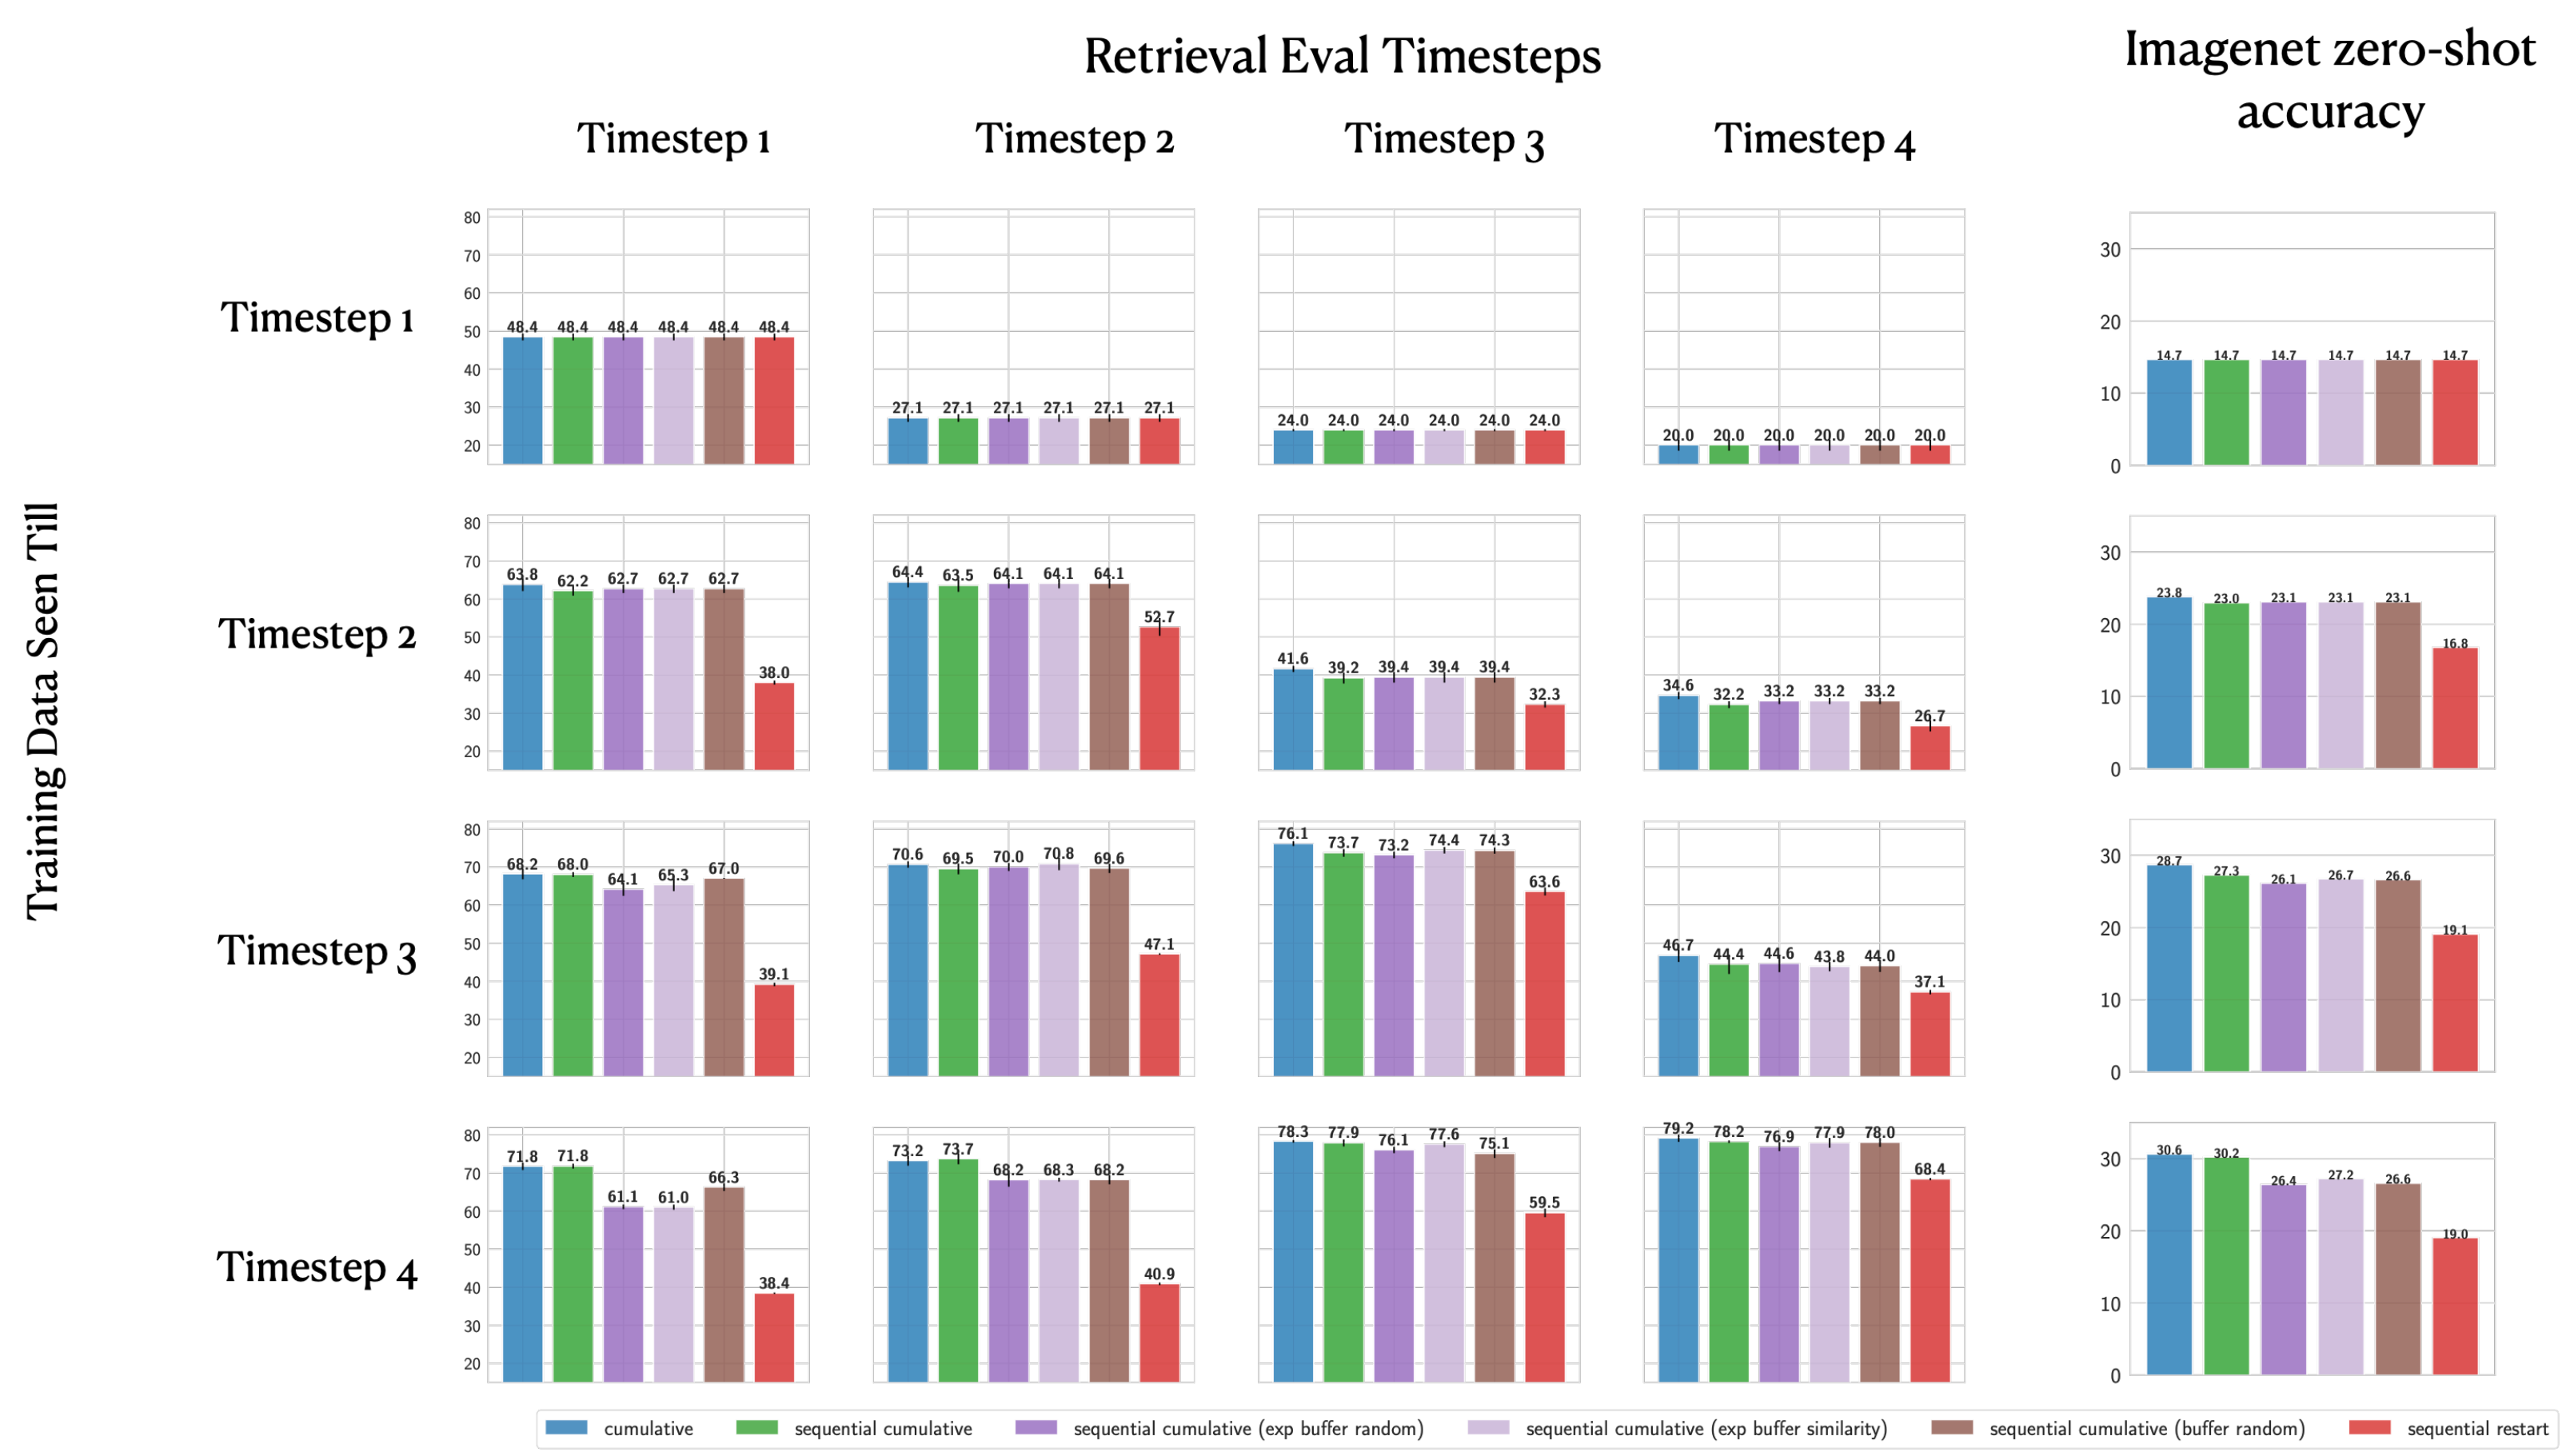} 
     \caption{}   
    \end{subfigure}
    \caption{YFCC 15M results}
    \label{fig:intro-figure}
\end{figure*}

\begin{figure*}[!t]
    \centering
    \begin{subfigure}[b]{\linewidth}
    \includegraphics[width=\linewidth]{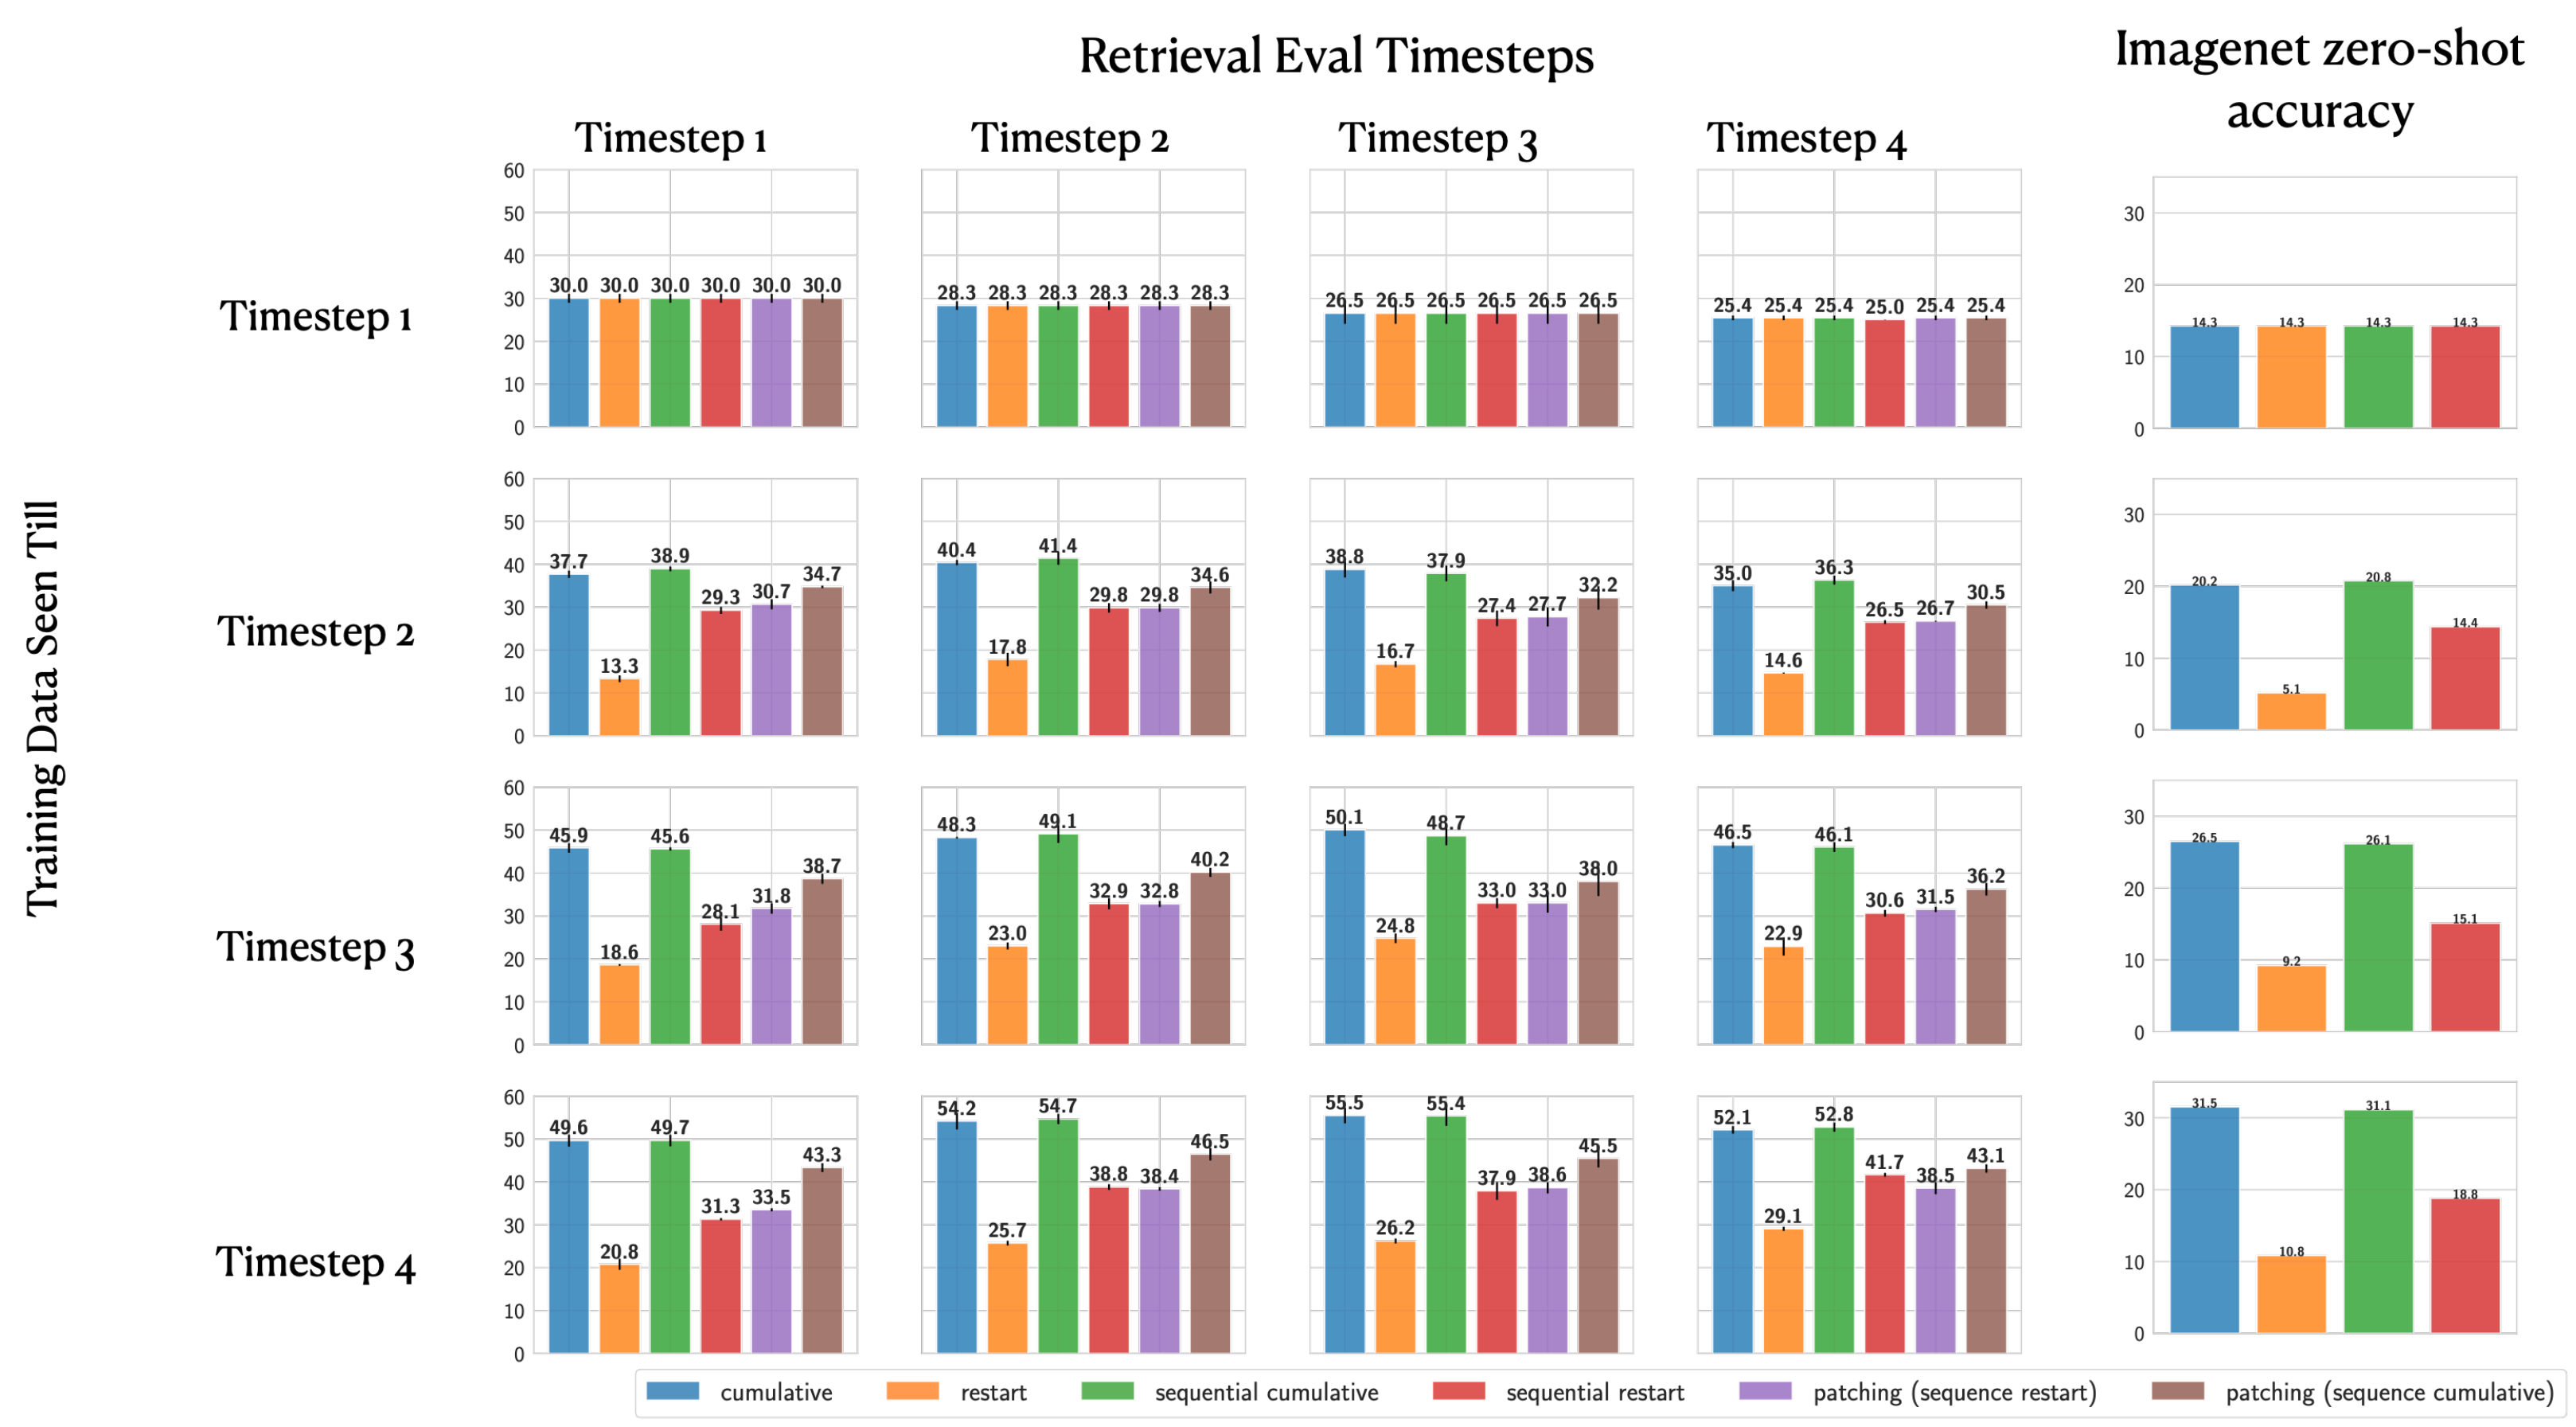} 
     \caption{}   
    \end{subfigure}
    \caption{YFCC 15M results}
    \label{fig:intro-figure}
\end{figure*}
